# Supplementary material for: Using Speech Foundational Models in Loss Functions for Hearing Aid Speech Enhancement
Source: arXiv:2407.13333 source file (2024-07-18)
Supplement: Supplementary file 1 [file appendix.tex]

\newpage
\newpage
\section{\textcolor{red}{DO NOT INCLUDE IN SUBMISSION}}

\begin{table}[!h]
    \centering
    \caption{Metric values for $\hat{s}$ (output of the denoiser $\mathcal{M}_\mathrm{D}$).}
    \begin{tabular}{cl|ccccc}
Dataset                  &Model                        &STOI      &PESQ      &SI-SNR    &fwSNR     \\
\hline
\multirow{4}{*}{\rotatebox[origin=c]{90}{CEC1}}&Unprocessed         &0.72      &1.10      &-4.61     &-0.92     \\
                         &$\mathcal{L}_{\mathrm{SNR}}$&0.76      &1.19      &3.31      &2.81      \\
                         &$\mathcal{L}_{\mathrm{WavLM}}$, Fine-tune&0.76      &1.20      &3.42      &2.51      \\
                         &$\mathcal{L}_{\mathrm{WavLM}}$, Scheduled&0.78      &1.23      &3.85      &0.73      \\
\hline
\multirow{4}{*}{\rotatebox[origin=c]{90}{CEC2}}&Unprocessed         &0.60      &1.16      &-10.69    &-3.22     \\
                         &$\mathcal{L}_{\mathrm{SNR}}$&0.67      &1.11      &-0.60     &-2.62     \\
                         &$\mathcal{L}_{\mathrm{WavLM}}$, Fine-tune&0.66      &1.10      &-0.71     &-2.66     \\
                         &$\mathcal{L}_{\mathrm{WavLM}}$, Scheduled&0.68      &1.12      &-0.35     &-2.44     \\

    \end{tabular}
    \label{tab:den_results}
\end{table}

\begin{table}[!h]
    \centering
    \resizebox{\columnwidth}{!}{%
    \begin{footnotesize}
    \caption{Metric values for $\hat{s}$ (output of the denoiser $\mathcal{M}_\mathrm{D}$).}
    \begin{tabular}{cc|ccccc}
        Stage                         &Model                         &HASPI     &STOI      &PESQ      &SI-SNR    &fwSNR     \\
\hline
denoised                      &noisy                         &0.47      &0.72      &1.10      &-4.61     &-0.92     \\
denoised                      &SNR                     &0.42      &0.76      &1.19      &3.31      &2.81      \\
denoised                      &WavLMTwostage            &0.42      &0.76      &1.20      &3.42      &2.51      \\
denoised                      &WavLMScheduled           &0.44      &0.78      &1.23      &3.85      &0.73      \\
\hline
amplified                     &noisy                         &0.47      &0.72      &1.10      &-4.61     &-0.92     \\
amplified                     &SNR                     &0.65      &0.68      &1.10      &-21.06    &1.86      \\
amplified                     &WavLMTwostage            &0.64      &0.69      &1.09      &-20.81    &1.41      \\
amplified                     &WavLMScheduled           &0.65      &0.71      &1.10      &-20.89    &-1.09     \\
\bottomrule     
    \end{tabular}
    \end{footnotesize}
    }
    \label{tab:den_results}
\end{table}

\begin{table}[]
    \centering
    \caption{Correlations in greyscale}
    \resizebox{\columnwidth}{!}{%
    \begin{footnotesize}
    \begin{tabular}{c|ccccccc}
         Scores    &\ac{HSI}             &$-\mathcal{L}_\mathrm{WLM}$&$-\mathcal{L}_\mathrm{SNR}$&SI-SNR         &HASPI          &STOI           &PESQ           \\
\hline
\ac{HSI}       &\cellcolor[gray]{0.50}1.00           &\cellcolor[gray]{0.71}0.58           &\cellcolor[gray]{0.85}-0.30          &\cellcolor[gray]{1.00}0.00           &\cellcolor[gray]{0.77}0.46           &\cellcolor[gray]{0.65}0.69           &\cellcolor[gray]{0.69}0.62           \\
$-\mathcal{L}_\mathrm{WLM}$&\cellcolor[gray]{0.71}0.58           &\cellcolor[gray]{0.50}1.00           &\cellcolor[gray]{0.85}-0.29          &\cellcolor[gray]{0.94}-0.12          &\cellcolor[gray]{0.76}0.48           &\cellcolor[gray]{0.66}0.69           &\cellcolor[gray]{0.63}0.74           \\
$-\mathcal{L}_\mathrm{SNR}$&\cellcolor[gray]{0.85}-0.30          &\cellcolor[gray]{0.85}-0.29          &\cellcolor[gray]{0.50}1.00           &\cellcolor[gray]{0.87}0.25           &\cellcolor[gray]{0.96}-0.08          &\cellcolor[gray]{0.86}-0.29          &\cellcolor[gray]{0.84}-0.31          \\
SI-SNR         &\cellcolor[gray]{1.00}0.00           &\cellcolor[gray]{0.94}-0.12          &\cellcolor[gray]{0.87}0.25           &\cellcolor[gray]{0.50}1.00           &\cellcolor[gray]{0.92}0.15           &\cellcolor[gray]{0.90}0.20           &\cellcolor[gray]{0.97}0.05           \\
HASPI          &\cellcolor[gray]{0.77}0.46           &\cellcolor[gray]{0.76}0.48           &\cellcolor[gray]{0.96}-0.08          &\cellcolor[gray]{0.92}0.15           &\cellcolor[gray]{0.50}1.00           &\cellcolor[gray]{0.68}0.65           &\cellcolor[gray]{0.72}0.57           \\
STOI           &\cellcolor[gray]{0.65}0.69           &\cellcolor[gray]{0.66}0.69           &\cellcolor[gray]{0.86}-0.29          &\cellcolor[gray]{0.90}0.20           &\cellcolor[gray]{0.68}0.65           &\cellcolor[gray]{0.50}1.00           &\cellcolor[gray]{0.59}0.82           \\
PESQ           &\cellcolor[gray]{0.69}0.62           &\cellcolor[gray]{0.63}0.74           &\cellcolor[gray]{0.84}-0.31          &\cellcolor[gray]{0.97}0.05           &\cellcolor[gray]{0.72}0.57           &\cellcolor[gray]{0.59}0.82           &\cellcolor[gray]{0.50}1.00           \\

    \end{tabular}
    \end{footnotesize}
    }
\end{table}

\begin{table}[]
    \centering
    \caption{Correlations in red}
    \resizebox{\columnwidth}{!}{%
    \begin{footnotesize}
    \begin{tabular}{c|ccccccc}
        {}    &{}             &\multicolumn{2}{c}{Losses}&SI-         & {}          &{}           &{}           \\
        \multirow{-2}{*}{Scores}    &\multirow{-2}{*}{\ac{HSI}}             &-$\mathcal{L}_{\mathrm{WLM}}$&-$\mathcal{L}_{\mathrm{SNR}}$&SNR         &\multirow{-2}{*}{HASPI}          &\multirow{-2}{*}{STOI}           &\multirow{-2}{*}{PESQ}          \\
\hline
\ac{HSI}             &\cellcolor[rgb]{1, 0.50, 0.50}1.00           &\cellcolor[rgb]{1, 0.64, 0.64}0.58           &\cellcolor[rgb]{1, 0.93, 0.93}-0.30          &\cellcolor[rgb]{1, 0.83, 0.83}0.00           &\cellcolor[rgb]{1, 0.68, 0.68}0.46           &\cellcolor[rgb]{1, 0.60, 0.60}0.69           &\cellcolor[rgb]{1, 0.63, 0.63}0.62           \\
-$\mathcal{L}_{\mathrm{WLM}}$&\cellcolor[rgb]{1, 0.64, 0.64}0.58           &\cellcolor[rgb]{1, 0.50, 0.50}1.00           &\cellcolor[rgb]{1, 0.93, 0.93}-0.29          &\cellcolor[rgb]{1, 0.87, 0.87}-0.12          &\cellcolor[rgb]{1, 0.67, 0.67}0.48           &\cellcolor[rgb]{1, 0.60, 0.60}0.69           &\cellcolor[rgb]{1, 0.59, 0.59}0.74           \\
-$\mathcal{L}_{\mathrm{SNR}}$&\cellcolor[rgb]{1, 0.93, 0.93}-0.30          &\cellcolor[rgb]{1, 0.93, 0.93}-0.29          &\cellcolor[rgb]{1, 0.50, 0.50}1.00           &\cellcolor[rgb]{1, 0.75, 0.75}0.25           &\cellcolor[rgb]{1, 0.86, 0.86}-0.08          &\cellcolor[rgb]{1, 0.93, 0.93}-0.29          &\cellcolor[rgb]{1, 0.94, 0.94}-0.31          \\
SI-SNR         &\cellcolor[rgb]{1, 0.83, 0.83}0.00           &\cellcolor[rgb]{1, 0.87, 0.87}-0.12          &\cellcolor[rgb]{1, 0.75, 0.75}0.25           &\cellcolor[rgb]{1, 0.50, 0.50}1.00           &\cellcolor[rgb]{1, 0.78, 0.78}0.15           &\cellcolor[rgb]{1, 0.77, 0.77}0.20           &\cellcolor[rgb]{1, 0.82, 0.82}0.05           \\
HASPI          &\cellcolor[rgb]{1, 0.68, 0.68}0.46           &\cellcolor[rgb]{1, 0.67, 0.67}0.48           &\cellcolor[rgb]{1, 0.86, 0.86}-0.08          &\cellcolor[rgb]{1, 0.78, 0.78}0.15           &\cellcolor[rgb]{1, 0.50, 0.50}1.00           &\cellcolor[rgb]{1, 0.62, 0.62}0.65           &\cellcolor[rgb]{1, 0.64, 0.64}0.57           \\
STOI           &\cellcolor[rgb]{1, 0.60, 0.60}0.69           &\cellcolor[rgb]{1, 0.60, 0.60}0.69           &\cellcolor[rgb]{1, 0.93, 0.93}-0.29          &\cellcolor[rgb]{1, 0.77, 0.77}0.20           &\cellcolor[rgb]{1, 0.62, 0.62}0.65           &\cellcolor[rgb]{1, 0.50, 0.50}1.00           &\cellcolor[rgb]{1, 0.56, 0.56}0.82           \\
PESQ           &\cellcolor[rgb]{1, 0.63, 0.63}0.62           &\cellcolor[rgb]{1, 0.59, 0.59}0.74           &\cellcolor[rgb]{1, 0.94, 0.94}-0.31          &\cellcolor[rgb]{1, 0.82, 0.82}0.05           &\cellcolor[rgb]{1, 0.64, 0.64}0.57           &\cellcolor[rgb]{1, 0.56, 0.56}0.82           &\cellcolor[rgb]{1, 0.50, 0.50}1.00           \\

    \end{tabular}
    \end{footnotesize}
    }
\end{table}

\begin{table}[]
    \centering
    \resizebox{\columnwidth}{!}{%
    \begin{footnotesize}
    \begin{tabular}{c|ccccccc}
         Scores    &\ac{HSI}             &$-\mathcal{L}_\mathrm{WLM}$&$-\mathcal{L}_\mathrm{SNR}$&SI-SNR         &HASPI          &STOI           &PESQ           \\
\hline
\ac{HSI}       &\cellcolor[gray]{0.50}1.00           &\cellcolor[gray]{0.71}0.58           &\cellcolor[gray]{0.85}-0.30          &\cellcolor[gray]{1.00}0.00           &\cellcolor[gray]{0.77}0.46           &\cellcolor[gray]{0.65}0.69           &\cellcolor[gray]{0.69}0.62           \\
$-\mathcal{L}_\mathrm{WLM}$&{}            &\cellcolor[gray]{0.50}1.00           &\cellcolor[gray]{0.85}-0.29          &\cellcolor[gray]{0.94}-0.12          &\cellcolor[gray]{0.76}0.48           &\cellcolor[gray]{0.66}0.69           &\cellcolor[gray]{0.63}0.74           \\
$-\mathcal{L}_\mathrm{SNR}$&{}            &{}            &\cellcolor[gray]{0.50}1.00           &\cellcolor[gray]{0.87}0.25           &\cellcolor[gray]{0.96}-0.08          &\cellcolor[gray]{0.86}-0.29          &\cellcolor[gray]{0.84}-0.31          \\
SI-SNR         &{}            &{}            &{}            &\cellcolor[gray]{0.50}1.00           &\cellcolor[gray]{0.92}0.15           &\cellcolor[gray]{0.90}0.20           &\cellcolor[gray]{0.97}0.05           \\
HASPI          &{}            &{}            &{}            &{}            &\cellcolor[gray]{0.50}1.00           &\cellcolor[gray]{0.68}0.65           &\cellcolor[gray]{0.72}0.57           \\
STOI           &{}            &{}            &{}            &{}            &{}            &\cellcolor[gray]{0.50}1.00           &\cellcolor[gray]{0.59}0.82           \\
PESQ           &{}            &{}            &{}            &{}            &{}            &{}            &\cellcolor[gray]{0.50}1.00           \\
    \end{tabular}
    \end{footnotesize}
    }
\end{table}

\begin{table}[]
    \centering
    \caption{Denoiser results inc HASPI}
    \begin{tabular}{cc|ccccc}
         Dataset                  &Model                        &HASPI    &STOI     &PESQ     &$\Delta$SI-SNR&$\Delta$fwSNR\\
\hline
\multirow{4}{*}{CEC1}                         &$\mathcal{L}_{\mathrm{SNR}}$&0.90      &0.76      &1.19      &7.92      &3.72      \\
                         &$\mathcal{L}_{\mathrm{WLM}}$, Fine-tune&0.90      &0.76      &1.20      &8.03      &3.42      \\
                         &$\mathcal{L}_{\mathrm{WLM}}$, Scheduled&0.91      &0.78      &1.23      &8.45      &1.65      \\
\hline
\multirow{4}{*}{CEC2}                         &$\mathcal{L}_{\mathrm{SNR}}$&0.72      &0.67      &1.11      &10.09     &0.60      \\
                         &$\mathcal{L}_{\mathrm{WLM}}$, Fine-tune&0.72      &0.66      &1.10      &9.98      &0.57      \\
                         &$\mathcal{L}_{\mathrm{WLM}}$, Scheduled&0.75      &0.68      &1.12      &10.33     &0.78      \\
    \end{tabular}
\end{table}

\begin{table}[!h]
    \centering
    \caption{Metric values for $\hat{s}$ (output of the denoiser $\mathcal{M}_\mathrm{D}$).}
    \begin{tabular}{cl|ccccc}
Data                  &Model                        &$\Delta$STOI      &$\Delta$PESQ      &$\Delta$SI-SNR    &$\Delta$fwSNR     \\
\hline
\multirow{3}{*}{\rotatebox[origin=c]{90}{CEC1}}                         &$\mathcal{L}_{\mathrm{SNR}}$&0.04      &0.08      &7.92      &\textbf{3.72}      \\
                         &$\mathcal{L}_{\mathrm{WLM}}$, FT&0.04      &0.10      &8.03      &3.42      \\
                         &$\mathcal{L}_{\mathrm{WLM}}$, Sched.&\textbf{0.07}      &\textbf{0.13}      &\textbf{8.45}      &1.65      \\
\hline
\multirow{3}{*}{\rotatebox[origin=c]{90}{CEC2}}                         &$\mathcal{L}_{\mathrm{SNR}}$&0.07      &-0.05     &10.09     &0.60      \\
                         &$\mathcal{L}_{\mathrm{WLM}}$, FT&0.06      &-0.05     &9.98      &0.57      \\
                         &$\mathcal{L}_{\mathrm{WLM}}$, Sched.&\textbf{0.08}      &\textbf{-0.04}     &\textbf{10.33}     &\textbf{0.78}      \\
    \end{tabular}
    \label{tab:den_results}
\end{table}
